# Supplementary material for: AI-Assisted Cervical Cancer Screening
Source: arXiv:2403.11936 source file (2024-09-04)
Supplement: Supplementary file 1 [file supplementary.tex]

\begin{document}
\title{Supplementary Material}
\section{Annotation Platform Visualization}
\sec
\end{document}
